# Supplementary material for: The Unreasonable Effectiveness of the Final Batch Normalization Layer
Source: arXiv:2109.09016 source file (2021-09-18)
Supplement: Supplementary file 1 [file appendix.tex]

\section{Appendix}
\setcounter{table}{0}
\setcounter{figure}{0}

\subsection{Additional Experiments}
In addition to the aforementioned experiments, we ran more tests to further support our findings:
%using one plant type as majority and the other one as a minority class, 
Turning off the bias at the final dense layer when the final BN layer is added, removing the final BN layer in inference time, using SeLU~\cite{klambauer2017self} instead of BN in the last layer, freezing and unfreezing the previous BN layers, label smoothing, training different CNN and NN from scratch rather than utilizing SOTA architectures, and using CIFAR-10\cite{krizhevsky2014cifar} and histopathological cancer datasets (to identify metastatic cancer in small image patches taken from larger digital pathology scans)\cite{veeling2018rotation}.

\subsection{Transfer Learning}

In simple terms, Transfer Learning is “leveraging the knowledge of a neural network learned by training on one task to apply it for another task.”  In other words, the learned weights of a model that was pre-trained on one data set are used to ‘bootstrap’ training of early or all but the final layer of a modified version of the model applied to a different data set. This technique allows faster training, whereby the model just learns the weights of the last fully connected layers, then applies a low learning rate finely tuned adjustment to the entire model’s weights.

For example, if the goal is for building an image classification application where the target images to be classified are similar to those present in established data sets such as ImageNet and CIFAR10/100, it makes sense to start of training using pre-trained neural-net models on these data sets, instead of doing it from scratch. 

This is achieved by two main concepts: Freezing and fine-tuning. It is a common strategy to freeze the layers in neural-networks that are supposed to be leveraged from the pre-trained model as is and no weight updates are expected on these layers. This is done keeping in mind, that contributions from these layers areas similar to those which would have been if the new network was being trained off from the ground. For example, the first few layers of any image-classifier would learn edges and patterns. So it makes sense to keep these frozen in most of the cases.

Unlike freezing, fine-tuning would mean allowing weight updates to happen. In other words, these layers are unfrozen or unlocked and they would participate in the transfer-learning process, but with one difference: These layers would now be initialized with the weights of the pre-trained neural network model rather than starting from some random initializer/ zero weights. This matters significantly, as convergence would be affected with the right set of weights which wouldn’t be the case if the network was being trained from scratch.

In this study, in order to fine-tune VGG19 and ResNet-34 architectures with PlantVillage dataset, the final classification layer is replaced with Adaptive Average Pooling (GAP), Batch-Norm, Dropout, Dense, ReLU, Batch-Norm and Dropout followed by the Dense and ReLU layer again. We borrowed this architecture from \textit{fastai} \footnote{https://www.fast.ai/} library that simplifies training fast and accurate neural nets using modern best practices.

\subsection{PlantVillage Dataset and Initial Modelling Efforts}

PlantVillage image data set has 54,306 images of 14 crop species with 26 diseases.  Table~\ref{tab:pv_full} summarizes this data set. In total, there are 38 different classes, and out of 54,306 images, there are 42,237 images in train set and 10,566 images in the validation set.

\begin{table}[ht]
\centering
\caption{PlantVillage dataset original sample sizes}
\label{tab:pv_full}
\begin{tabular}{llll}
\toprule
Plant                       & Class                                   & Train & Validation \\ \midrule
Tomato    & Bacterial\_spot                         & 1702  & 425        \\
                            & Early\_blight                           & 800   & 200        \\
                            & Late\_blight                            & 1403  & 353        \\
                            & Leaf\_Mold                              & 761   & 191        \\
                            & Septoria\_leaf\_spot                    & 1417  & 354        \\
                            & Spider\_mites Two-spotted\_spider\_mite & 1341  & 335        \\
                            & Target\_Spot                            & 1123  & 281        \\
                            & Tomato\_Yellow\_Leaf\_Curl\_Virus       & 4286  & 1071       \\
                            & Tomato\_mosaic\_virus                   & 299   & 74         \\
                            & healthy                                 & 1272  & 318        \\ \midrule
Apple      & Apple\_scab                             & 504   & 126        \\
                            & Black\_rot                              & 496   & 125        \\
                            & Cedar\_apple\_rust                      & 220   & 55         \\
                            & healthy                                 & 1316  & 329        \\\midrule
Blueberry                   & healthy                                 & 1202  & 300        \\\midrule
Cherry                      & Powdery\_mildew                         & 842   & 210        \\\midrule
Corn       & healthy                                 & 684   & 170        \\
                            & Cercospora\_leaf\_spot Gray\_leaf\_spot & 355   & 91         \\
                            & Common\_rust\_                          & 953   & 239        \\
                            & Northern\_Leaf\_Blight                  & 697   & 173        \\
                            & healthy                                 & 16    & 5          \\\midrule
Grape     & Black\_rot                              & 944   & 236        \\
                            & Esca\_(Black\_Measles)                  & 1107  & 276        \\
                            & Leaf\_blight\_(Isariopsis\_Leaf\_Spot)  & 861   & 215        \\
                            & healthy                                 & 339   & 84         \\\midrule
Orange                      & Haunglongbing\_(Citrus\_greening)       & 4405  & 1102       \\\midrule
Peach      & Bacterial\_spot                         & 1838  & 459        \\
                            & healthy                                 & 288   & 72         \\\midrule
Pepper     & Bacterial\_spot                         & 797   & 200        \\
                            & healthy                                 & 1181  & 295        \\\midrule
Potato     & Early\_blight                           & 800   & 200        \\
                            & Late\_blight                            & 800   & 200        \\
                            & healthy                                 & 121   & 31         \\
Raspberry                   & healthy                                 & 297   & 74         \\\midrule
Soybean                     & healthy                                 & 4072  & 1018       \\\midrule
Squash                      & Powdery\_mildew                         & 1448  & 365        \\\midrule
Strawberry & Leaf\_scorch                            & 886   & 222        \\
                            & healthy                                 & 364   & 92        \\ \bottomrule
\end{tabular}
\end{table}

See Table~\ref{tab:pv_stats} for the number of images in each plant type and class. All the plant classes other than healthy ones are put under unhealthy class of the respective plant type. 

\begin{table}[h]
\centering
\caption{PlantVillage dataset class distributions}
\label{tab:pv_stats}
\begin{tabular}{lllll}
\toprule
\multicolumn{1}{c}{Plant type} & \multicolumn{2}{c}{Train set} & \multicolumn{2}{c}{Validation set} \\ 
           & Healthy       & Unhealthy      & Healthy         & Unhealthy         \\ \midrule
Potato     & 121           & 1600           & 31              & 400               \\ 
Peach      & 288           & 1838           & 72              & 459               \\ 
Cherry     & 684           & 842            & 170             & 210               \\ 
Grape      & 339           & 2912           & 84              & 727               \\ 
Tomato     & 1272          & 13132          & 318             & 3284              \\ 
Pepper     & 1181          & 797            & 295             & 200               \\ 
Corn       & 16            & 2005           & 5               & 503               \\ 
Orange     & 0             & 4405           & 0               & 1102              \\ 
Blueberry  & 1202          & 0              & 300             & 0                 \\ 
Apple      & 1316          & 1220           & 329             & 306               \\ 
Squash     & 0             & 1448           & 0               & 365               \\ 
Soybean    & 4072          & 0              & 1018            & 0                 \\ 
Raspberry  & 297           & 0              & 74              & 0                 \\ 
Strawberry & 364           & 886            & 92              & 222               \\ \bottomrule
\end{tabular}
\end{table}

We at first used the entire PlantVillage dataset in Table~\ref{tab:pv_full} and trained with ResNet-34 architecture for 38 classes. Using scheduled learning rates, we obtained 99.782\% accuracy after 10 epochs. This is already better than what the researchers of PlantVillage project got as 99.34\% with GoogleNet. This result clearly shows that we can build a reliable state-of-the-art classifier just by using a ResNet architecture (pre-trained on ImageNet dataset) without much effort. The training metrics for that model can be found in Table~\ref{tab:pv_resnet}.

\begin{table}[h]
\centering
\caption{Training metrics for a 38-class ResNet34 model trained for 10 epochs on PlantVillage dataset.}
\label{tab:pv_resnet}
\begin{tabular}{lllll}
Epoch      & Train Loss & Validation Loss & Accuracy & Error Rate \\\toprule
0          & 0.3304   & 0.1448        & 0.9525 & 0.0474   \\
1          & 0.1749   & 0.0732        & 0.9758 & 0.0241   \\
2          & 0.1066   & 0.0422        & 0.9859 & 0.0140   \\
3          & 0.0742   & 0.0311        & 0.9903 & 0.0096   \\
4          & 0.0499   & 0.0278        & 0.9907 & 0.0092   \\
5          & 0.0476   & 0.0261        & 0.9920 & 0.0079   \\
6          & 0.0299   & 0.0190        & 0.9935 & 0.0064   \\
7          & 0.0098   & 0.0086        & 0.9973 & 0.0026   \\
8          & 0.0053    & 0.0076        & 0.9975 & 0.0024   \\
9          & 0.0067    & 0.0074        & \textbf{0.9978} & 0.0021  \\
\bottomrule
\end{tabular}
\end{table}

Then using the binary classes depicted in Table~\ref{tab:pv_stats}, we trained another model for binary classification and obtained 99.91\% accuracy after 10 epochs. That is, we can predict 9,991 out of 10,000 images correctly. The training metrics for that model can be found in Table~\ref{tab:pv_resnet_binary}. It’s important to note that we didn’t even do any fine tuning or any other laborious work. This also indicates that the PlantVillage data set is noise free.

\begin{table}[h]
\centering
\caption{Training metrics for a 2-class (healthy vs unhealthy regardless of plant type) ResNet34 model trained for 10 epochs on PlantVillage dataset.}
\label{tab:pv_resnet_binary}
\begin{tabular}{lllll}
Epoch       & Train Loss & Validation Loss & Accuracy & Error Rate \\\toprule
0           & 0.0893    & 0.0369    & 0.9873 & 0.0126    \\
1           & 0.0391    & 0.0145    & 0.9956 & 0.0043    \\
2           & 0.0133    & 0.0073    & 0.9978 & 0.0021    \\
3           & 0.0137    & 0.0054    & 0.9981 & 0.0018    \\
4           & 0.0112    & 0.0049    & 0.9982 & 0.0017    \\
5           & 0.0094    & 0.0051    & 0.9979 & 0.0020    \\
6           & 0.0134    & 0.0040    & 0.9983 & 0.0016    \\
7           & 0.0154    & 0.0034    & 0.9987 & 0.0011     \\
8           & 0.0095    & 0.0030    & 0.9988 & 0.0011    \\
9           & 0.0058    & 0.0025    & \textbf{0.9991} & 0.0008     \\
\bottomrule
\end{tabular}
\end{table}

In order to simulate rare events in agriculture, we randomly picked 1,000 healthy and 10 unhealthy samples from a plant type for the training set, 150 healthy and 7 unhealthy samples for the validation set, and 150 samples from both classes for the test set. For details, see Table~\ref{tab:sample_dist}.

\begin{table}[h]
\centering
\caption{Class distributions for the imbalanced data set that we used during our experiments for the final BN layer.}
\label{tab:sample_dist}
\resizebox{\columnwidth}{!}{
\begin{tabular}{lcccccc}
 & \multicolumn{2}{c}{Train set} & \multicolumn{2}{c}{Validation set} & \multicolumn{2}{c}{Test set} \\ \toprule
 & \multicolumn{1}{l}{Unhealthy} & \multicolumn{1}{l}{Unhealthy} & Healthy         & Unhealthy         & Healthy      & Unhealthy      \\ \midrule
Apple  & 1,000 & 10 & 150 & 7 & 150 & 150 \\
Pepper & 1,000 & 10 & 150 & 7 & 150 & 150 \\ 
Tomato & 1,000 & 10 & 150 & 7 & 150 & 150 \\ \bottomrule
\end{tabular}}
\end{table}

\subsection{Adding the Final BN Layer}

\begin{figure*}[h]
\includegraphics[width=\textwidth]{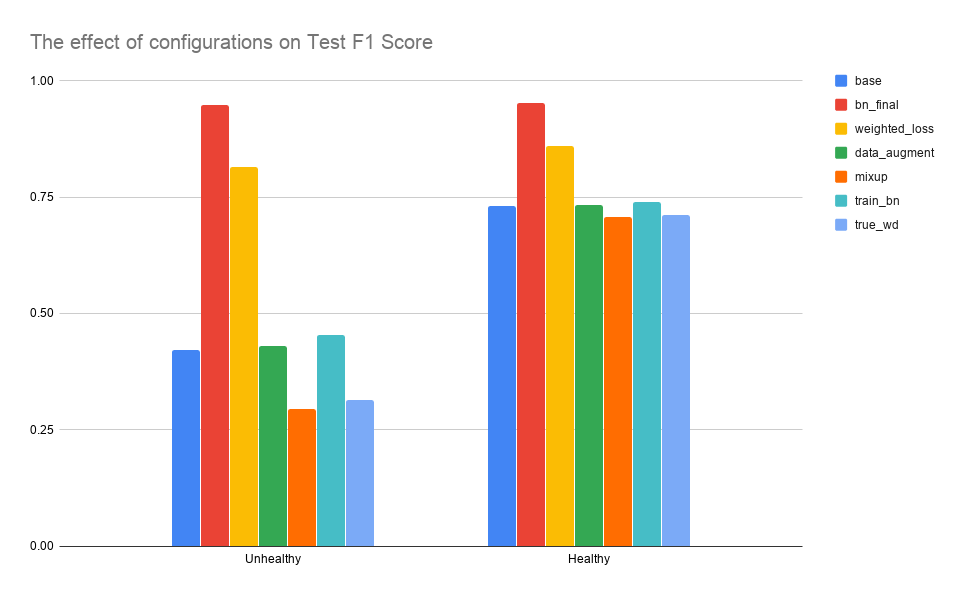}
\caption{The highest gain in test F1 score for both classes is achieved by adding a final BN layer (only one parameter is set to True at a time).(i.e. test F1 score is increased from 0.42 to 0.95 for minority class (unhealthy) just by adding a final BN layer in ResNet34)}
\label{fig:bn_barchart}
\end{figure*}

In order to see what the model actually sees during training, we visualized the activations on the final CNN layer. Usually, the heatmaps generated are not class-discriminative, i.e.~they only correspond to activations generated in the forward pass through the network. Selvaraju et al.~\cite{selvaraju2017grad} devised a way to visualize which parts of an input image result in the prediction of a specific class. In this study, we used this approach to generate class-discriminative heatmaps. Looking at Figure~\ref{fig:activations}, we see that the model without final BN layer looks at the wrong part of the picture while predicting. The highlighted parts (heatmap) basically tell us which parts of an image induced the wrong classification. In this example, the model made the wrong prediction because of the highlighted part.

%\begin{figure}[h]
%\includegraphics[width=\textwidth]{figures/activations.png}
%\caption{Class discriminative activations while predicting}
%\label{fig:activations}
%\end{figure}

\begin{figure}
\begin{subfigure}{0.5\textwidth}
\includegraphics[width=1.0\linewidth]{figures/activations_bn_false.png}
\subcaptionbox{\textbf{Final BN = False.} Wrong prediction. The activations for unhealthy class is glowing on the wrong pixels and it is predicted as healthy as the glowing parts look healthy (clean). The probability of being unhealthy is 36\% (we some some minor activations close to defected parts). There is no activation happening for healthy class.\label{fig:actbnfalse}}[.9\linewidth]

\end{subfigure}
\begin{subfigure}{0.5\textwidth}
\includegraphics[width=1.0\linewidth]{figures/activations_bn_true.png}
\subcaptionbox{\textbf{Final BN = True.} Correct prediction by a close margin ( 51\%). The activations for unhealthy class is glowing on the right pixels and it is predicted as unhealthy as the glowing parts look unhealthy (defects). The activations for healthy class is also glowing on the right pixels but still shows some defects.\label{fig:actbntrue}}[.9\linewidth]

\end{subfigure}
\caption{Class-discriminate activations for an unhealthy Apple leaf during prediction.}
\label{fig:activations}
\end{figure}

\begin{figure*}
\includegraphics[width=\textwidth, scale=0.5]{figures/withBN_confident.png}
\caption{The activations and class probabilities from a model with final BN. The probabilities of belonging to a class are leveled off around 50\%.}
\label{fig:withoutBN_confident}
\end{figure*}

Here are some of the observations we had during experimenting under different settings:
\begin{itemize}

\item We tested adding the final BN layer approach with ISIC Skin Cancer data set under the same class imbalance settings, and the test F1 score for malignant class is increased from 0.06 to 0.37.

\item Replacing RELU in head layers with SELU activation function didn't make any significant change with the final BN layer added.

\item We investigated if the effect of final BN layer only happens on the classes having similar features (i.e. both Apples or Peppers and the only difference is some blights or spots on the leaves), and we trained a model on two different plants in the same imbalance (i.e. 1,000 Apple samples and 10 Pepper samples).  It turns out that final BN layer is still useful for the minority class. It reduced the test F1 score for majority class but increased test F1 score for minority class with a less confidence in both validation and test set. It is also surprising that we were able to predict all of samples in test set from the minority class, 150/150, with just 8 epochs.

\item We investigated if the effect of final BN layer only happens in state-of-the-art CNN architectures and we built a simple model with 2 CNN layers and no BN layer at all. Then we added a final BN layer to see its effect on loss curves. We observed that the training gets smoother and model generalizes better.

\item Due to its regularization effect, it is usually advised that BN layer and dropout shouldn't be used at the same time. To test this, we removed the dropout layer from the head, and then added final BN layer again. As a result, adding the final BN layer and removing the dropout layer from head layers boosted the test set performance by 2-3\%.

\item Since BN layer already includes the additional bias term, it makes no sense to add another bias term in the convolution layer as well as in the dense layer. Simply speaking, BN shifts the activation by their mean values. Hence, any constant will be canceled out. In default ResNet-34 architecture, all the biases preceding BN layers are all turned off by default. Given that, we removed the bias in the dense layer preceding the final BN as well and we gained 2-3\% boost in F1. This is probably because we reduced the complexity of the network a little bit by turning of the last bias. In a small network, it is clear that we need a bias in the nodes, but in a large network, removing it makes almost no difference. Since there are already two dense layers and 2 BN layers in the head, we tested to remove bias from both after adding the final BN layer, but the result was unexpectedly worse. It didn't converge till 20th epoch, minority validation turned out to be zero and test F1 score was 14\%. So the claim that bias is not required in a dense layer if it is located behind BN layer is not valid for our settings.

\item Label smoothing is a loss function modification that has been shown to be very effective for training deep learning networks~\cite{muller2019does}. It changes the training target for the NN from a hard ‘1’ to ‘1-label smoothing adjustment’, meaning the NN is trained to be a bit less confident of it’s answers. The default value is usually .1, meaning the target answer is .9 (1 minus .1) and not 1.
NN’s have a bad habit of becoming ‘over-confident’ in their predictions during training, and this can reduce their ability to generalize and thus perform as well on new, unseen future data. In addition, large data sets can often include incorrectly labeled data, meaning inherently the NN should be a bit skeptical of the ‘correct answer’ to reduce extreme modeling around some degree of bad answers. Even though it resonates well and sounds promising for our use case, no significant impact has been observed during our experiments using label smoothed cross entropy as a loss function.

\begin{figure*}
\includegraphics[width=\textwidth, scale=0.5]{figures/withoutBN_confident.png}
\caption{The activations and class probabilities from a model having no final BN. As can be seen on upper left corner, \textit{unhealthy} leaf in the validation set is predicted as \textit{healthy} and the probability of being \textit{healthy} is 91\%. The model is highly confident even if it is wrong. This is an expected behaviour of DNN.}
\label{fig:withoutBN_confident}
\end{figure*}

\item As mentioned before, neural networks are often over-confident and poorly calibrated relative to their true accuracy. A network should provide a calibrated confidence measure in addition to its prediction~\cite{guo2017calibration}. In other words, the probability associated with the predicted class label should reflect its ground truth correctness likelihood. Given this, we also evaluated our approach with respect to calibration effect and found out that a network with the final BN layer is more calibrated and has lower Brier score (see Figure~\ref{fig:ece}).

\end{itemize}

\begin{figure*}
\includegraphics[width=\textwidth, scale=0.8]{figures/calibration.png}
\caption{With the final BN layer, a network has much lower ECE (Expected Calibration Error), i.e. has a more ideal confidence relative to its own accuracy. It also has the lower the Brier score indicating that the predictions are calibrated. In effect, a final BN layered network is not ‘over-confident’ and as a result generalizes and performs better on live future data.}
\label{fig:ece}
\end{figure*}

\subsection{Development Environment}

We run our experiments on GPU-supported Colab\footnote{https://colab.research.google.com/} server provided by Google . The GPU details can be seen at Figure~\ref{fig:gpu}.

\begin{figure*}
\includegraphics[width=\textwidth, scale=0.5]{figures/colab_gpu.png}
\caption{GPU specifications provided free on Colab server by Google.}
\label{fig:gpu}
\end{figure*}
